# Supplementary material for: Demonstration of a Reconfigurable Entangled Radiofrequency-Photonic Sensor Network
Source: arXiv:1910.08825 source file (2020-04-21)
Supplement: Supplementary file 1 [file RF_Entangled_Sensors_SM_Final.pdf]

# Supplemental Material

## Demonstration of a Reconfigurable Entangled Radiofrequency-Photonic Sensor Network

Yi Xia<sup>#,1</sup>, Wei Li<sup>#,2,\*</sup>, William Clark,<sup>3</sup> Darlene Hart,<sup>4</sup> Quntao Zhuang,<sup>5,1</sup> and Zheshen Zhang<sup>2,1,†</sup>

<sup>1</sup>*James C. Wyant College of Optical Sciences, University of Arizona, Tucson, Arizona 85721, USA*

<sup>2</sup>*Department of Materials Science and Engineering,  
University of Arizona, Tucson, Arizona 85721, USA*

<sup>3</sup>*General Dynamics Mission Systems, 8220 East Roosevelt Street, Scottsdale, Arizona 85257, USA*

<sup>4</sup>*General Dynamics Mission Systems, 9 Vreeland Road, Florham Park, New Jersey 07932, USA*

<sup>5</sup>*Department of Electrical and Computer Engineering,  
University of Arizona, Tucson, Arizona 85721, USA*

### I. THEORETICAL FRAMEWORK

We present a detailed theoretical framework for performance analysis. In Section I A, we analyze the single sensor performance and explain the transformation of RF signals into optical displacements. In Section I B, we analyze the performance of a network of sensors with shared continuous-variable (CV) multipartite entanglement and solve the optimum entanglement configuration. In Section I C, we explain an alternative resource counting method and compare the entangled scheme with the optimal separable scheme subject to the photon-number constraint. In Section I D, we connect the measurement results to the parameters of a RF field.

#### A. Single RF-photonic sensor enhanced by squeezed light

We consider an entangled RF-photonic sensor network composed of  $M$  sensors. The quantum states of interest at each sensor are carried on three optical spectral modes, i.e., a central mode  $\hat{a}_c^{(m)}$  at the optical carrier frequency  $\Omega$  and two sideband modes  $\hat{a}_{\pm}^{(m)}$  at optical frequencies  $\Omega \pm \omega_c$ . Here,  $1 \leq m \leq M$  indexes the sensors. Suppose the probed RF field at the  $m$ -th sensor is represented by the waveform  $\mathcal{E}_m(t) = E_m \cos(\omega_c t + \varphi_m)$ , where  $\omega_c$  is the carrier frequency of the RF field,  $E_m$  is the RF-field amplitude, and  $\varphi_m$  is the RF-field phase. The EOM transduces the RF field into a phase modulation on the optical field so that the spectral mode  $\hat{a}_\omega e^{-i\omega t}$  at  $\omega$  becomes

$$\hat{a}_\omega e^{-i\omega t} e^{i\zeta E_m \cos(\omega_c t + \varphi_m)} = \hat{a}_\omega \sum_{n=-\infty}^{\infty} i^n J_n(A_m) e^{i(-\omega - n\omega_c)t + n\varphi_m}, \quad (\text{S1})$$

where the Jacobi-Anger expansion has been employed,  $J_n(z)$  is the  $n$ -th Bessel function of the first kind. Here  $A_m = \zeta E_m$ , where  $\zeta = \pi\gamma/V_\pi$  accounts for the RF-to-photonic conversion efficiency and the conversion from an external electric field to the applied voltage on the EOM by an antenna as modeled by  $\gamma$ . Effectively, the spectral mode  $\hat{a}_\omega$  undergoes a frequency-domain beam splitter transform and is spread over to the spectral modes  $\omega - n\omega_c$ ,  $n = 0, \pm 1, \pm 2, \dots$ . For small  $A_m$ ,  $J(A_m) \sim (A_m)^n 2^{-n}/n!$  decays quickly with  $n$ . In a weak RF-field scenario, only the  $n = 0, \pm 1$  components need be considered such that  $\hat{a}^{(m)}$ 's undergo an effective frequency-domain beam splitter transform, yielding the transformed spectral mode operators

$$\begin{aligned} \hat{a}_c^{(m)'} &= J_0(A_m)\hat{a}_c^{(m)} + iJ_1(A_m)\hat{a}_-^{(m)}e^{i\varphi_m} + iJ_1(A_m)\hat{a}_+^{(m)}e^{-i\varphi_m} \\ \hat{a}_+^{(m)'} &= J_0(A_m)\hat{a}_+^{(m)} + iJ_1(A_m)\hat{a}_c^{(m)}e^{i\varphi_m} + iJ_1(A_m)\hat{a}_-^{(m)}e^{-i\varphi_m} \\ \hat{a}_-^{(m)'} &= J_0(A_m)\hat{a}_-^{(m)} + iJ_1(A_m)\hat{a}_c^{(m)}e^{i\varphi_m} + iJ_1(A_m)\hat{a}_+^{(m)}e^{-i\varphi_m}, \end{aligned} \quad (\text{S2})$$

where  $\hat{a}_{2\pm}^{(m)}$  are higher-order spectral modes at frequencies  $\Omega \pm 2\omega_c$ , and  $J_{-n}(z) = (-1)^n J_n(z)$  has been used. Initially, all the sideband modes  $\hat{a}_{\pm}^{(m)}, \hat{a}_{2\pm}^{(m)}$  are in zero-mean states, while the central spectral mode  $\hat{a}_c^{(m)}$  is in a quantum state close to the coherent state  $|\alpha_m\rangle$ . Thus,  $\langle \hat{a}_{\pm}^{(m)'} \rangle = iJ_1(A_m)e^{\pm i\varphi_m}\alpha_m$ .

The optical field operator carrying the three spectral modes at sensor  $m$  now reads

$$\hat{E}^{(m)}(t) = \hat{a}_c^{(m)'} e^{-i\Omega t} + \hat{a}_+^{(m)'} e^{-i(\Omega + \omega_c)t} + \hat{a}_-^{(m)'} e^{-i(\Omega - \omega_c)t}. \quad (\text{S3})$$

Let the LO optical field be  $E_{\text{LO}}^{(m)}(t) = E_{\text{LO}} e^{-i(\Omega t + \theta)}$ , where  $E_{\text{LO}}$  is real. The balanced homodyne measurement generates a photocurrent

$$\begin{aligned} I(t) &= \text{Re} \left[ \hat{E}^{(m)} E_{\text{LO}}^{(m)*} \right] \\ &= \text{Re} \left[ E_{\text{LO}} e^{i\theta} (\hat{a}_c^{(m)'} + \hat{a}_+^{(m)'} e^{-i\omega_c t} + \hat{a}_-^{(m)'} e^{i\omega_c t}) \right], \end{aligned} \quad (\text{S4})$$

where we have set the electron charge  $q = 1$  for theoreti-

\* Current address: Department of Electronic and Information Engineering, Shanxi University, Taiyuan, China

† zsz@email.arizona.edu

# Equal contributions

cal convenience.

An electronic mixer supplied by an RF LO at  $\omega_c$  and with a phase  $\phi_0$  is then applied on the photocurrent, i.e.  $\cos(\omega_c t + \phi_0)$ , moving the photocurrent's spectral component at  $\omega_c$  to the baseband. After filtering, the baseband photocurrent reads

$$I_B^{(m)}(t) = -\text{Re} \left[ e^{i\theta} \hat{b}^{(m)'} \right], \quad (\text{S5})$$

where we have defined the mode

$$\hat{b}^{(m)'} \equiv (e^{i\phi_0} \hat{a}_+^{(m)'} + e^{-i\phi_0} \hat{a}_-^{(m)'}) / \sqrt{2}. \quad (\text{S6})$$

In doing so, one only needs to consider measurements on the effective mode  $\hat{b}^{(m)'}$  in estimating the parameters of the probed RF field. Likewise, a corresponding effective mode before the RF-to-photonic transduction is defined as

$$\hat{b}^{(m)} \equiv (e^{i\phi_0} \hat{a}_+^{(m)} + e^{-i\phi_0} \hat{a}_-^{(m)}) / \sqrt{2}. \quad (\text{S7})$$

Derived from Eq. S2, the transform of the effective mode through the transduction is

$$\hat{b}^{(m)'} = J_0(A_m) \hat{b}^{(m)} + i \sqrt{2} J_1(A_m) \cos(\phi_0 + \varphi_m) \hat{a}_c^{(m)} + \text{v.c.}, \quad (\text{S8})$$

where v.c. are the vacuum modes and higher order zero-mean modes. For  $A_m \ll 1$  and  $|\alpha_m| \gg 1$ , the evolution of  $\hat{b}_m$  through the transduction is well described by a first-order approximation, giving a displacement of  $i \sqrt{2} J_1(A_m) \cos(\phi_0 + \varphi_m) \alpha_m$  on  $\hat{b}_m$  on the phase quadrature. Thus, to access the displacement, the LO phase needs to be set to  $\theta = \pi/2$  to observe the phase quadrature of  $\hat{b}^{(m)}$ , i.e.,  $I_B^{(m)}(t) = \text{Im} [\hat{b}^{(m)'}]$ , as experimentally verified by the sinusoidal signal in Fig. 2 of the main text. Moreover, because the RF-field information is transferred to the phase quadrature of the effective mode, a quantum enhancement in the measurement sensitivity requires that the effective mode is in a phase squeezed state. This is achieved by setting the OPA to operate in a parametric amplification regime.

To measure a RF-field phase  $\varphi_m \ll 1$ , we set  $\phi_0 = \mp \pi/2$ , then the effective mode, up to the leading order, becomes

$$\hat{b}^{(m)'} = J_0(A_m) \hat{b}^{(m)} + g_m i \sqrt{2} J_1(A_m) \varphi_m \hat{a}_c^{(m)} + \text{v.c.}, \quad (\text{S9})$$

where  $g_m = \pm 1$  can be tuned by the sign of  $\phi_0$ . Here if we further expand  $J_1(A_m) \simeq A_m/2 = \pi \frac{\gamma E_m}{2V_\pi}$  and replace  $\hat{a}_c^{(m)}$  with its mean  $a_c^{(m)}$ , the second term becomes  $i \pi g_m \sqrt{2} a_c^{(m)} \frac{\gamma E_m}{2V_\pi} \varphi_m$ , i.e., a displacement on the phase quadrature. This expression also agrees with Eq. (2) in the main text.

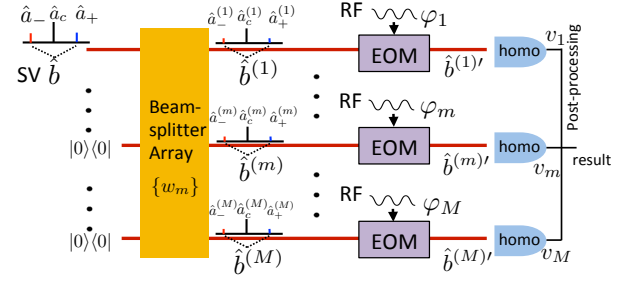

FIG. S1. Theoretical model for the entangled RF-photonic sensor network. SV: squeezed vacuum. EOM: electro-optic modulator. homo: homodyne measurement. At the quantum source, the sideband modes  $\hat{a}_\pm$  are entangled in a two-mode squeezed state, leading to the effective mode  $\hat{b} = i(\hat{a}_+ - \hat{a}_-) / \sqrt{2}$  in a phase SV state. The central spectral mode  $\hat{a}_c$  is close to a coherent state  $|\alpha\rangle$ . A beam splitter array with weights  $\{w_m, 1 \leq m \leq M\}$  generates the CV multipartite entangled state of the effective modes  $\{\hat{b}^{(m)}, 1 \leq m \leq M\}$ . Each  $\hat{b}^{(m)} = i(\hat{a}_+^{(m)} - \hat{a}_-^{(m)}) / \sqrt{2}$  accounts for two sideband modes. The EOM transduces the RF signal into optical field quadrature displacements. Postprocessing of homodyne measurement results at all sensors generates a sum with weights  $\{v_m, 1 \leq m \leq M\}$ , which is used to infer the average RF-field amplitude or the AoA.

## B. Entangled RF-photonic sensor network

Shown in Fig. S1, to apply the DQS protocol developed in Ref. [S1] to an entangled RF-photonic sensor network, the quantum source first effectively generates a single-mode squeezed vacuum mode  $\hat{b} = i(\hat{a}_+ - \hat{a}_-) / \sqrt{2}$ , where  $\hat{a}_\pm$  are the sideband modes. Subsequently, a beam splitter array with weights  $\{w_m, 1 \leq m \leq M\}$  ( $\sum w_m^2 = 1$ ) produces the modes  $\hat{b}^{(m)} = i(\hat{a}_+^{(m)} - \hat{a}_-^{(m)}) / \sqrt{2}$  that are distributed to different sensors. In the experiment, such a state is produced with a two-mode squeezed vacuum state between the sideband modes  $\hat{a}_\pm$  such that  $\langle \hat{a}_+ \hat{a}_- \rangle = \sqrt{N_S(N_S + 1)} e^{i\tau}$  and  $\langle \hat{a}_+^2 \rangle = \langle \hat{a}_-^2 \rangle = 0$ , where  $N_S$  is the mean photon number. The variance of the phase quadrature  $\langle \text{Im} [\hat{b}]^2 \rangle = (2N_S + 1 - 2 \cos \tau \sqrt{N_S(N_S + 1)})/4$ . Choosing  $\tau = 0$ , the variance is minimized to

$$\langle \text{Im} [\hat{b}]^2 \rangle = \frac{1}{4} \frac{1}{(\sqrt{N_S} + \sqrt{N_S + 1})^2}, \quad (\text{S10})$$

so that a squeezed vacuum state is generated at the effective mode  $\hat{b}$ .

In the beam splitter array, all spectral modes undergo the same transform. Thus, the central spectral modes  $\hat{a}_c^{(m)}$  at different sensors are also generated by splitting the central spectral mode  $\hat{a}_c$  at the source. Prior to the EOM at each sensor,  $\hat{b}^{(m)} = w_m \hat{b} + \text{v.c.}$ ,  $\hat{a}_c^{(m)} = w_m \hat{a}_c + \text{v.c.}$ , and

the effective mode after the EOM becomes

$$\hat{b}^{(m)'} = J_0(A_m)w_m\hat{b} + g_m w_m i \sqrt{2}J_1(A_m)\varphi_m\hat{a}_c + \text{v.c.}, \quad (\text{S11})$$

on which the phase quadrature  $I_B^{(m)}(t) = \text{Im}[\hat{b}^{(m)'}]$  is measured.

Suppose the global parameter to be estimated is  $\bar{\varphi} = \sum_m c_m \varphi_m$ , with weights being  $c_m$  real. To obtain an estimation, a suitable set of  $w_m$ 's is required, and postprocessing on measurement outcomes of all sensors is further needed to construct an unbiased estimator

$$\hat{L} = s \sum_m v_m I_B^{(m)}(t) = s \text{Im} \left[ \sum_m v_m \hat{b}^{(m)'} \right], \quad (\text{S12})$$

where the weights  $v_m$  are real and normalized,  $\sum_m v_m^2 = 1$ , and  $s > 0$  is a scaling factor. The unbiased condition requires the expectation value

$$\langle \hat{L} \rangle = s \sum_m v_m g_m w_m \varphi_m \beta = \sum_m c_m \varphi_m, \quad (\text{S13})$$

where  $\sqrt{2}J_1(A_m)\alpha = \beta$  is fixed. Thus, the chosen  $v_m, w_m$ 's need to make  $c_m = s g_m v_m w_m \beta, \forall m$ .

To use the phase squeezed state in the  $\hat{b}$  mode to minimize the variance of the estimator,  $v_m = w_m$  is needed, and consequently the optimum choices of the parameters are

$$w_m^{\text{opt}} = \frac{\sqrt{|c_m|}}{\sqrt{\sum |c_m|}}, g_m^{\text{opt}} = \text{sign}(c_m), s^{\text{opt}} = \sum |c_m|/\beta. \quad (\text{S14})$$

The minimum variance is thus

$$\text{var}(\hat{L})^{\text{opt}} = \left( \sum |c_m|/\beta \right)^2 \langle \text{Im}[\hat{b}]^2 \rangle, \quad (\text{S15})$$

where the variance of the phase squeezed state is given by Eq. S10.

To show that the weights  $w_m^{\text{opt}}$ 's indeed yield the optimum entanglement-enhanced estimation performance, we choose a set of sub-optimum weights  $\{w_m, 1 \leq m \leq M\}$  and the associated postprocessing weights  $\{v_m, 1 \leq m \leq M\}$  to maintain an unbiased estimator, as specified in Eq. S13. The estimator variance is then derived as following. Denote the effective modes as  $\hat{b}' = (\hat{b}^{(1)'}, \dots, \hat{b}^{(M)'} )^T$ , obtained from a beam splitter transform  $\mathbf{T} = (w, \mathbf{T}_1)$  on mode  $\hat{b}$  and vacuum modes  $\hat{e} = (\hat{e}_2, \dots, \hat{e}_M)$ . Here,  $w \equiv (w_1, \dots, w_M)^T$ , i.e.,  $\hat{b}' = (w, \mathbf{T}_1)(\hat{b}, \hat{e})^T$ . From the orthogonality condition,  $\mathbf{T}^T \mathbf{T} = \mathbf{T} \mathbf{T}^T = \mathbf{I}_M$ , one has  $w^T w = 1, w^T \mathbf{T}_1 = 0, \mathbf{T}_1^T \mathbf{T}_1 = \mathbf{I}_{M-1}$ , and  $w w^T + \mathbf{T}_1 \mathbf{T}_1^T = \mathbf{I}_{M-1}$ . Here,  $\mathbf{I}_L$  is an  $L \times L$  identity matrix. Let  $v = (v_1, \dots, v_M)^T$ , the estimator is then written as  $\hat{L} = s \text{Im} [v^T \mathbf{T}(\hat{b}, \hat{e})^T]$ . Thus,

the variance of the estimator

$$\begin{aligned} \text{var}(\hat{L}) &= s^2 v^T \mathbf{T} \text{Diag} \left[ \langle \text{Im}[\hat{b}]^2 \rangle, \frac{1}{4} \mathbf{I}_{M-1} \right] \mathbf{T}^T v \\ &= s^2 (v^T w)^2 \langle \text{Im}[\hat{b}]^2 \rangle + \frac{1}{4} s^2 v^T \mathbf{T}_1 \mathbf{T}_1^T v \\ &= s^2 (v^T w)^2 \left( \langle \text{Im}[\hat{b}]^2 \rangle - \frac{1}{4} \right) + \frac{1}{4} s^2 v^T v \\ &= \frac{1}{\beta^2} \left[ \left( \sum_{m=1}^M g_m c_m \right)^2 \left( \langle \text{Im}[\hat{b}]^2 \rangle - \frac{1}{4} \right) + \frac{1}{4} \left( \sum_{m=1}^M \frac{c_m^2}{w_m^2} \right) \right], \end{aligned} \quad (\text{S16})$$

where  $v^T w = \sum_{m=1}^M g_m c_m / s \beta$  and  $v^T v = \sum_{m=1}^M c_m^2 / (s^2 w_m^2 \beta^2)$  have been used. Again, the variance of the phase squeezed state is given in Eq. S10. To rederive the optimum parameters  $w_m$ 's and  $g_m$ 's, the constraint  $\sum_{m=1}^M w_m^2 = 1$  is considered. Using Lagrangian multipliers, it becomes easy to see that  $w_m \propto \sqrt{|c_m|}$ . Also, since  $\langle \text{Im}[\hat{b}]^2 \rangle - \frac{1}{4} \leq 0$  due to squeezing,  $g_m = \text{sign}(c_m)$  is needed. The same solution as in Eq. S14 for the optimum parameters is then derived.

The above analysis applies to an ideal lossless situation. In a practical scenario, however, loss  $1 - \eta$  is present at each sensor. Effectively, loss can be accounted for at the source by replacing Eq. S10 with

$$\langle \text{Im}[\hat{b}]^2 \rangle = \frac{1}{4} \left[ \frac{\eta}{(\sqrt{N_S} + \sqrt{N_S + 1})^2} + (1 - \eta) \right], \quad (\text{S17})$$

where  $\eta$  is the transmissivity. The optimum solutions in Eq. S14 and Eq. S15, as well as the variance in Eq. S16 remains valid with  $\beta = \sqrt{\eta} \sqrt{2}J_1(A_m)\alpha$ .

### C. Performance analysis

To compare the performance of quantum sensing protocols, one should first identify the resource constraints. Various theoretical works simply consider an energy constraint, i.e., by fixing the total mean photon numbers employed in different protocols under comparison. The energy constraint is valid in scenarios where the interrogated sample is sensitive to the probe power caused by, e.g., photodamage or self-concealing. In RF-photonics sensing and LIGO, however, the optical power should ideally be cranked up as much as one can until the device power accommodation limit is arrived. Therefore, in an RF-photonics sensor, the power carried by the central mode  $\hat{a}_c$  needs be large, subject to the operational limit of the device. For example, integrated RF-photonics sen-

sors can accommodate milliwatts of optical power [S2]. In a classical separable RF-photonic sensor network, the effective mode  $\hat{b}$  is in a vacuum state, and the laser power distribution to different sensors is optimized through tuning the beam-splitter ratios.

In an entangled RF-photonic sensor network, phase squeezed light resides in the effective mode  $\hat{b}$ . Because the experimental energy the squeezed state  $N_S \ll |\alpha|^2$ , it is negligible, as compared to that of the central spectral mode. As such, the performance comparison between the classical separable and entangled sensor networks is based on setting the classical scheme's  $\hat{b}$  in a vacuum state and the entangled scheme's  $\hat{b}$  to a squeezed state while employing identical energies on the central spectral modes for both cases. The estimation variances for both schemes are modeled by Eq. S15, with  $\langle \text{Im}[\hat{b}]^2 \rangle$  given in Eq. S17 for the entangled sensor network and  $\langle \text{Im}[\hat{b}]^2 \rangle = 1/4$  for the classical separable sensor network.

To show that the quantum state shared by the sensors is indeed entangled, we performed a theoretical comparison between the DQS scheme and the optimum separable scheme, subject to a total photon number constraint in the  $\hat{b}_m$  modes for both cases. As analyzed in Ref. [S1, S3], in the absence of loss, the optimum separable DQS utilizes  $\{\hat{b}^{(m)}, 1 \leq m \leq M\}$  modes in a product of squeezed vacuums, with the optimum mean photon number distribution  $N_S^{(m)}$  under the constraint  $\sum_{m=1}^M N_S^{(m)} = N_S$ . Suppose the same beam splitter array is used to distribute the central spectral mode's coherent state to different sensors, the unbiased estimator condition remains the same as Eq. S13. Now, the  $\hat{b}^{(m) \prime}$  modes are separable, each having a variance of

$$\text{var}(\text{Im}[\hat{b}^{(m) \prime}]) = \frac{1}{4} \left[ \frac{\eta}{\left( \sqrt{N_S^{(m)}} + \sqrt{N_S^{(m)} + 1} \right)^2} + (1 - \eta) \right]. \quad (\text{S18})$$

Akin to Eq. S16, the estimation variance

$$\text{var}(\hat{L}) = \sum_{m=1}^M \frac{c_m^2}{w_m^2 \beta^2} \text{var}(\text{Im}[\hat{b}^{(m) \prime}]). \quad (\text{S19})$$

For a set of fixed  $w_m$ 's, one optimizes  $N_S^{(m)}$  to minimize the estimation variance. One can show the overall minimum is achieved at  $w_m^2 \propto c_m \sqrt{\text{var}(\text{Im}[\hat{b}^{(m) \prime}])}$ :

$$\text{var}(\hat{L})^* = \min_{\sum_m N_S^{(m)} = N_S} \sum_{m=1}^M \frac{c_m}{\beta} \sqrt{\text{var}(\text{Im}[\hat{b}^{(m) \prime}])}. \quad (\text{S20})$$

In our experiment, at the source we measured the anti-

squeezing level as  $\sim 10$  dB above the shot-noise level and the squeezing level as  $\sim 4$  dB below the shot-noise level, from which we can infer the ideal source squeezing as  $\sim 11.7$  dB and mean photon number  $N_S \sim 3.3$ . In the field amplitude measurement, the measured squeezing was  $\sim 3.2$  dB (noise variance  $\sim 0.48$  of that of the shot noise) for the three sensor network case. Thus, the overall efficiency  $\eta \sim 0.56$  are then derived. With equal weights, the optimum separable scheme employs  $\sim 7.9$  dB of squeezing at the local source, to match the total mean photon number in squeezing, and achieves a 2.7 dB of noise reduction (noise variance  $\sim 0.53$  of the shot noise). This leads to a  $\sim 10\%$  advantage in estimation variance for our experimental result over that of the optimum separable sensor network, thereby verifying the entanglement shared by the sensors.

It is worth noting that the optimum separable RF-photonic sensor network discussed above requires that each sensor has its own squeezed-light source, which induces a substantial resource overhead.

#### D. Finite difference method for the estimation of AoA of the RF field

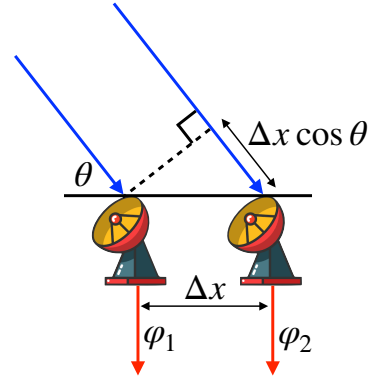

FIG. S2. A simple scheme to estimate the AoA of an incident RF field based on phase difference ( $\varphi_2 - \varphi_1$ ) measurement at two RF sensors. Dashed line is the wavefront of the RF field.

A simple example of measuring the AoA of an incident RF field is illustrated in Fig. S2. The AoA  $\theta$  is related to the relative phase of the two sensors by

$$\frac{\varphi_2 - \varphi_1}{2\pi} = \frac{\Delta x \cos \theta}{\lambda} + k, \quad (\text{S21})$$

where  $\lambda$  is the wavelength of the RF field, and  $k$  is an integer.  $k$  can be set to 0, if the sensors are located close to a less than a wavelength, i.e.,  $\Delta x/\lambda \ll 1$ , but the measurement of the AoA, in general, is not restricted to this

assumption. The AoA can then be estimated as

$$\theta = \arccos \frac{(\varphi_2 - \varphi_1)\lambda}{2\pi\Delta x}. \quad (\text{S22})$$

Since both  $\lambda$  and  $\Delta x$  are predetermined, the measurement of the AoA of an RF field is transformed into a difference phase estimation problem undertaken by the two sensors, which is a focus of the present article. Now we characterize the discretization error and optimize the precision of phase-difference estimation.

We will consider the three-point case,  $x_1 < x_2 < x_3$ , suppose the weights are  $c_1, c_2, c_3$ . The estimator is

$$\hat{L} = c_1\varphi(x_1) + c_2\varphi(x_2) + c_3\varphi(x_3). \quad (\text{S23})$$

*Case 1.*— Phase-difference estimation at a central node.

$$\begin{aligned} \varphi(x_1) &= \varphi(x_2) - \varphi^{(1)}(x_2)\Delta x + \frac{1}{2}\varphi^{(2)}(x_2)\Delta x^2 + O(\Delta x^3), \\ \varphi(x_3) &= \varphi(x_2) + \varphi^{(1)}(x_2)\Delta x + \frac{1}{2}\varphi^{(2)}(x_2)\Delta x^2 + O(\Delta x^3). \end{aligned} \quad (\text{S24})$$

One requires  $c_3 = 1 + c_1, c_2 = -1 - 2c_1$  to ensure the expectation value  $\langle \hat{L} \rangle = \varphi^{(1)}(x_2)\Delta x + O(\Delta x^2)$ . In particular if we require  $c_1 + c_3 = 0$ , or  $(c_1, c_2, c_3) = (-1/2, 0, 1/2)$ , then  $\langle \hat{L} \rangle = \varphi^{(1)}(x_2)\Delta x + O(\Delta x^3)$ .

With the proper chosen weights in Eq. S14, the variance in Eq. S15 is

$$\text{var}(\hat{L}) = \left( \sum |c_m|/\beta \right)^2 \langle \text{Re} \hat{b}^2 \rangle \propto (|c_1| + |1 + 2c_1| + |1 + c_1|)^2. \quad (\text{S25})$$

It is minimized when  $c_1 = -1/2$ . Thus, it is always optimum to use  $(c_1, c_2, c_3) = (-1/2, 0, 1/2)$ , because this minimizes both the estimation variance and the discretization error for the phase gradient.

*Case 2.*— Phase-difference estimation at an edge node.

$$\begin{aligned} \varphi(x_2) &= \varphi(x_1) + \varphi^{(1)}(x_1)\Delta x + \frac{1}{2}\varphi^{(2)}(x_1)\Delta x^2 + O(\Delta x^3), \\ \varphi(x_3) &= \varphi(x_1) + \varphi^{(1)}(x_1)2\Delta x + \frac{1}{2}\varphi^{(2)}(x_1)4\Delta x^2 + O(\Delta x^3). \end{aligned} \quad (\text{S26})$$

One requires  $c_2 = 1 - 2c_3, c_1 = c_3 - 1$  to ensure the expectation value  $\langle \hat{L} \rangle = \varphi^{(1)}(x_1)\Delta x + O(\Delta x^2)$ . If  $c_2 + 4c_3 = 0$  is required, then  $(c_1, c_2, c_3) = (-3/2, 2, -1/2)$  and  $\langle \hat{L} \rangle = \varphi^{(1)}(x_1)\Delta x + O(\Delta x^3)$ .

A similar analysis can be performed for the second-order derivative, except that there is only one possible set of parameters for each case. To estimate at a central node, one needs  $c_1 = c_3 = 1/2, c_2 = -1$ , so  $\langle \hat{L} \rangle = \varphi^{(2)}(x_2)\Delta x^2 + O(\Delta x^4)$ . To estimate at an edge

node, one needs  $c_1 = 1, c_2 = -2, c_3 = 1$ , so  $\langle \hat{L} \rangle = \varphi^{(2)}(x_1)\Delta x^2 + O(\Delta x^3)$ .

## II. EXPERIMENTAL DETAILS

Here, we provide more details about the experimental setup and the acquired data. Sec. II A introduces the components used in the experiment and the phase-locking mechanisms. Sec. II A provides data of the calibration of the shot-noise level, the electronic noise floor, and the squeezing level at different RF frequencies. Sec. II C elaborates the performance of each individual sensor at different input power levels and shows a nice agreement between the experimental data and a theoretical model.

### A. Detailed description of experimental setup

A detailed experimental diagram is drawn in Fig. S3. A 1550-nm mode-hop-free semiconductor laser (New Focus Velocity TLB-6728) generates  $\sim 10$  mW of light, which is modulated by a fiber-based phase modulator (PM) driven by a 24-MHz signal to create two sidebands for cavity locking based on the Pound-Drever-Hall (PDH) technique. The modulated light is subsequently boosted to  $\sim 1$  W by an erbium-doped fiber amplifier (EDFA) and coupled to free space. The 1550-nm light is first filtered by a locked 1550-nm mode-cleaning cavity (MC) and then split into two arms to serve, respectively, as the pump for second-harmonic generation (SHG) and the LO for homodyne measurements. The semi-monolithic SHG cavity entails a curved cavity mirror with 10% reflectivity at 775 nm and 94% reflectivity at 1550 nm [S4] and a type-0 periodically-poled KTiOPO<sub>4</sub> (PPKTP) crystal temperature stabilized at 34.0°C. The PPKTP crystal has a curved facet being highly reflective at 1550 nm and 775 nm and a flat facet that is anti-reflection coated at both wavelengths. The SHG cavity is locked using the 24-MHz sideband and generates  $\sim 300$  mW of 775-nm light under a 500-mW 1550-nm pump. The 775-nm light is first filtered by a locked 775-nm MC and then injected through a curved cavity mirror into an OPA cavity where a second identical PPKTP crystal temperature stabilized at 40.5°C is embedded. The curved mirror of the OPA cavity has 95% reflectivity at 775 nm and 87.5% reflectivity at 1550 nm. To generate phase squeezed light, a weak 1550-nm beam is tapped from the LO and modulated by a free-space PM to create 20-MHz sidebands. The modulated weak 1550-nm beam is reflected on a 775-nm/1550-nm dichroic beam splitter (DBS) and then

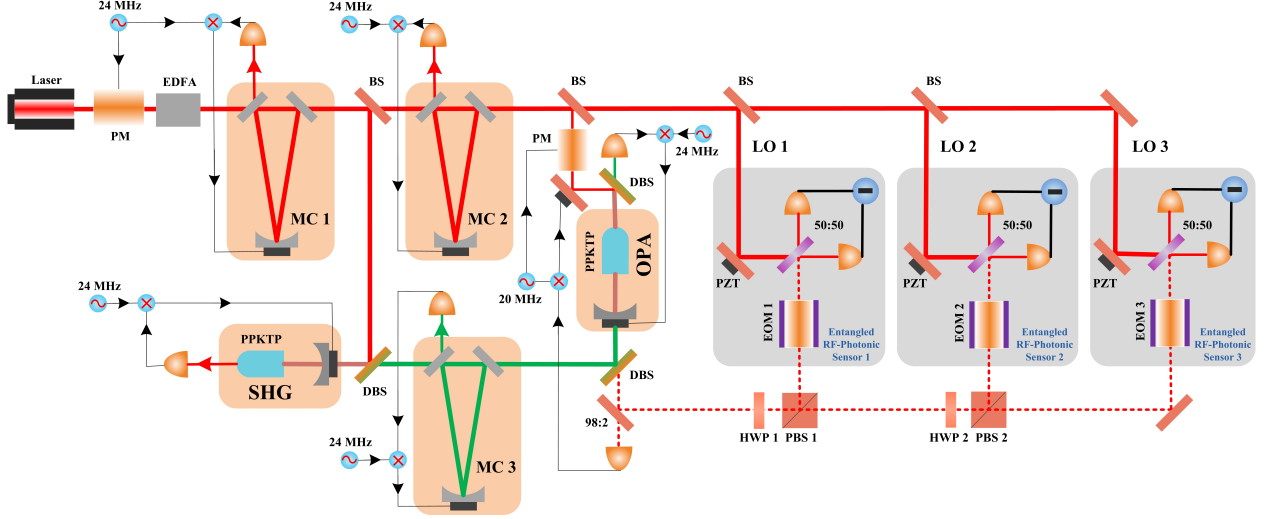

FIG. S3. Detailed experimental diagram. EOM: electro-optic modulator; MC: mode-cleaning cavity; BS: beam splitter; LO: local oscillator; DBS: Dichroic beam splitter; PPKTP: periodically-poled  $\text{KTiOPO}_4$ ; OPA: optical parametric amplifier; SHG: second-harmonic generation; PBS: polarizing beam splitter; PM: phase modulator; HWP: half-wave plate; PZT: piezoelectric transducer.

seeds the OPA cavity. The OPA cavity is locked by the 24-MHz sideband of the 775-nm light that transmits through the DBS. 2% of the 1550-nm output from the OPA curved cavity mirror is tapped and is employed to lock the phase between the 1550-nm seed beam and the 775-nm pump using the 20-MHz sidebands so that the OPA operates in a parametric amplification regime. When phase locked, the OPA cavity emits quantum light composed of an effective squeezed vacuum state residing in the 11-MHz sideband modes while the central spectral mode is a displaced phase squeezed state. Due to the large quadrature displacement, the central spectral mode can be well approximated by a classical coherent state. The single spatial-mode quantum light is diverted into three RF-phonic sensors by two variable beam splitters (VBSs), each consisting of a half-wave plate (HWP) and a polarizing beam splitter (PBS). The splitting ratios of both VBSs determines the CV multipartite entangled state. Each RF-phonic sensor is equipped with an EOM driven by the probed RF signal with 11-MHz carrier frequency. Due to the phase modulation, a portion of the coherent state in the central mode is transferred to quadrature displacement at the 11-MHz sidebands that accommodate the phase squeezed state. The magnitude of the quadrature displacement is dependent on the amplitude and phase of the probed RF field, as described by Eq. 1 of the main text and analyzed in Supplemental Information I. After the EOM, the quantum signal and the LO interfere on a 50:50 BS. By fine tuning the spot sizes of both beams, a classical interference

visibility in excess of 97% was achieved at each sensor. The two outputs of the BS are detected by two photodiodes, each with  $\sim 88\%$  quantum efficiency, in a balanced homodyne configuration. The difference photocurrent is amplified by a transimpedance amplifier with a gain of  $20 \times 10^3$  V/A. The DC component of the output voltage signal is utilized to lock the phase between the LO and the quantum signal so that the LO always addresses the squeezed phase quadrature with the displacement. The 11-MHz component of the voltage signal from each sensor is first demodulated by an electronic mixer, filtered by a 240-kHz low-pass filter, and recorded by an oscilloscope (LeCroy WaveRunner 8404 M) with a 4-GHz analog bandwidth (only 200 MHz bandwidth was used) at a 50 M Samples/s/channel sampling rate. Postprocessing derives the estimation and measurement noise variances.

## B. Calibration of shot-noise and squeezing levels

Prior to taking data, we first calibrated the shot-noise level and compared it with the electronic noise floor. To do so, a local oscillator with 14.1 mW power was fed to the homodyne detector of Sensor 1 while the signal input to the detector was blocked. Setting the resolution bandwidth of the RF spectrum analyzer to 300 kHz and the video bandwidth to 300 Hz, the noise power spectrum of the homodyne detector is found flat beyond 1.9 MHz, showing shot-noise limited behavior (red curve of Fig. S4). The measured shot-noise level agreed pre-

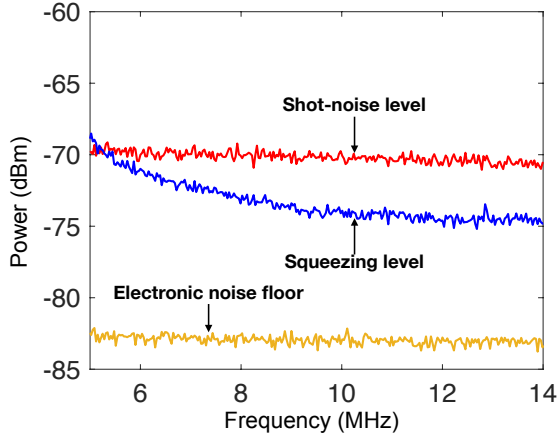

FIG. S4. Calibration of the shot-noise and squeezing levels. The shot-noise (squeezing) level is represented by the red (blue) curve, while the electronic noise floor is plotted in the yellow curve as a comparison. All measurements were taken with a resolution bandwidth of 300 kHz and a video bandwidth of 300 Hz.

cisely with a model that accounted for the local oscillator power, detector quantum efficiency, the gains of the amplifiers, and the resolution bandwidth of the RF spectrum analyzer. As a comparison, the electronic noise floor of the homodyne detector was measured by blocking the local oscillator and is depicted in the yellow curve in Fig. S4. The shot-noise level is 13 dB higher than the electronic noise floor, allowing for the observation of sub-shot-noise behavior enabled by squeezed light.

We then measured the squeezing level at different RF frequencies. In the measurement, the OPA was locked to operate in the parametric amplification regime to produce phase squeezed light, and the relative phase between the squeezed light and the local oscillator was locked to  $\pi/2$  so that the local oscillator was ensured to address the phase quadrature of the squeezed light. The measured squeezing level is plotted in the blue curve of Fig. S4. Sub-shot-noise behavior was observed at frequencies higher than  $\sim 5.5$  MHz. Squeezing was not observed at lower frequencies, likely due to the residue amplified spontaneous emission noise and the Brillouin scattering noise after the mode-cleaning cavities. Using mode-cleaning cavities with narrower linewidths, one may observe squeezing at lower frequencies. At 11 MHz, the carrier frequency of the probed RF field, the observed squeezing level was  $\sim 4$  dB, consistent with other experimental data.

### C. Performance of individual sensors

In the entangled sensor network, the three RF-photon sensors receive different portions of the original squeezed light, based on the splitting ratios of the VBSs determined by a specific distributed sensing task. To quantify the performance of each sensor at a certain input power level, the amount of noise power arising from the homodyne measurements is recorded under different input power levels. We first fix the splitting ratio of VBS 2 at 50:50 while varying the splitting ratio of VBS 1 from 0:100 to 100:0. In doing so, Sensor 1's received portion of the squeezed light varies from 0% to 100%, while Sensor 2 and Sensor 3 equally share the rest of the power. The resulting noise powers for the three sensors at different splitting ratios of VBS 1 are plotted in Fig. S5a. We then fix the splitting ratio of VBS 2 at 0:100 while varying the splitting ratio of VBS 1 from 100:0 to 0:100. In doing so, the squeezed light is split between Sensor 1 and Sensor 3 with different ratios, while Sensor 2 is unused. The corresponding noise powers for Sensor 1 and Sensor 2 are recorded and plotted in Fig. S5b. Finally, the splitting ratio of VBS 1 is fixed at 50:50, and that of VBS 2 is varied from 100:0 to 0:100. In this set of measurements, Sensor 1 always receives 50% of the squeezed light, while Sensor 2 and Sensor 3 share the rest 50% with various ratios. The noise powers for all three sensors at different splitting ratios are recorded and plotted in Fig. S5c. In all three sets of measurements, the experimental data are compared with a theoretical model, as depicted in the solid curves. Nice agreement between the theory and experimental data is found.

### D. Additional experimental data

#### 1. Phase-difference estimation at a central node

In addition to the data reported in the main text, we experimentally estimated the phase difference at a central node, served by Sensor 2. To do so, the weights for the optimum CV multipartite entangled state is  $[1/2, 0, -1/2]$ , generated by setting the splitting ratios of VBS 1 and 2 to 50:50 and 0:100. The AoA is emulated by an RF-field phase difference across the three sensors. The negative sign in the weights is introduced by adding a  $\pi$ -phase delay at Sensor 3. In the measurement, the RF phase at Sensor 1 is swept from 0.17 rad to -0.17 rad, and at the same time the RF phase at Sensor 2 is swept from -0.17 rad to 0.17 rad, while the RF-field amplitudes are set identical. The homodyne data from the three sensors are weighted to obtain an unbiased estimator. The estimated phase difference vs. the applied RF-field phase are plot-

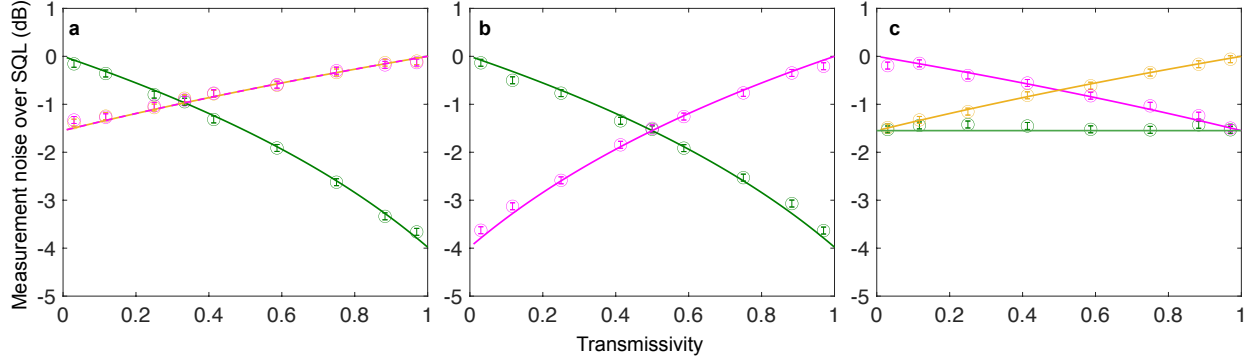

FIG. S5. The measurement noise powers at the three sensors under different input power levels, tuned by a VBS. (a) The splitting ratio of VBS 2 was fixed at 50:50 while that of VBS 1 was varied from 0:100 to 100:0. (b) The splitting ratio for VBS 2 was fixed at 0:100 while that of VBS 1 was varied from 100:0 to 0:100. (c) The splitting ratio of VBS 1 was fixed at 50:50 while that of VBS 2 was varied from 100:0 to 0:100. Experimental data are plotted in green circles for Sensor 1, gold circles for Sensor 2, and magenta circles for Sensor 3. Solid curves represent theoretical predictions. Error bars account for estimated uncertainties arising from experimental instabilities.

ted as blue circles in Fig. S6a and compared to the classical separable scheme (red triangles), with the shaded area representing the estimation uncertainties, showing a 3.5-dB reduction for the entangled case. Figure S6b plots the measurement noise and estimation variances at the two sensors in performing the phase-difference estimation at a central node.

## 2. Optimization of multipartite entangled state

In addition to optimizing the CV multipartite entangled state for estimating phase difference at an edge node, we also measured the estimation variances under different quantum circuit settings for the task of estimating the average RF-field amplitude and the task of estimating the phase difference at a central node. Fig. S7a plots the comparison on the estimation variances between the classical separable and entangled sensor networks. To optimize the CV multipartite entangled state, the splitting ratio for VBS 2 is fixed at 50:50 while the splitting ratio for VBS 1 is tuned from 100:0 to 0:100. The largest advantage for the entangled sensor network occurs at a transmissivity of 0.33 for VBS 1, when all sensors receive equal amount of optical power. The experimental data agree very well with the theoretical predictions represented by the solid lines (See Sec. II E for more details). In optimizing the CV multipartite entangled state for phase-difference estimation at a central node, the splitting ratio for VBS 2 is kept 0:100 while the splitting ratio for VBS 1 is tuned between 100:0 to 0:100. The negative sign in transmissivity represents a

sign flip on the homodyne data in postprocessing, as articulated in the main text. Fig. S7b plots a comparison on the estimation variances between the classical separable and entangled sensor networks in the task of phase-difference estimation at a central node. As discussed in the main text, the asymmetric behavior is a signature for the quantum correlations between the measurement noise at different sensors. The experimental data show nice agreement with our theoretical model.

## E. Theoretical model for the experiment

In the entangled RF-photon sensor network, let the global parameter to be estimated be a weighted average of the phase of the RF field at different sensors, i.e.,  $\bar{\varphi} = \sum_m c_m \varphi_m$ , with the weights  $c_m$ 's being real. Also the estimation of any analytical function of  $\varphi_m$ 's can be reduced to the estimation of weighted sum by linearization and adopting adaptivity [S5]. The average field-amplitude estimation problem can be formulated in a similar way. Under beam splitter ratios  $\{w_m\}$  for amplitude and  $\{g_m = \pm 1\}$  determined by RF phase delays at the sensors, the estimation variance can be derived as

$$\text{var} = \frac{1}{\beta^2} \left[ \left( \sum_{m=1}^M g_m c_m \right)^2 \delta_b + \frac{1}{4} \left( \sum_{m=1}^M \frac{c_m^2}{w_m^2} \right) \right].$$

Here,  $\beta$  is a coefficient determined by the mean photon number of the baseband light, the transduction efficiency of the EOM, and the system efficiency.  $\delta_b \equiv \eta \langle \text{Im} [\hat{b}]^2 \rangle - \eta/4$ , with  $\langle \text{Im} [\hat{b}]^2 \rangle$  being the variance of the

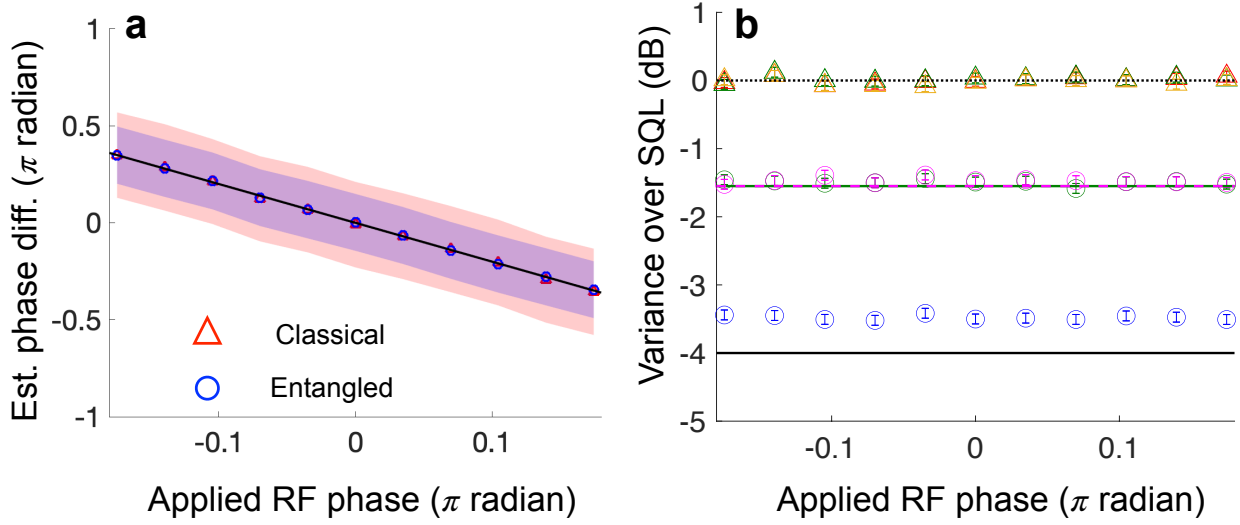

FIG. S6. (a) Estimation of phase difference at a central node. Circles: data for entangled sensors; triangles: data for classical separable sensors. Shaded area: estimation uncertainties for the entangled (blue) and classical separable (red) sensor networks. The entangled sensor network show a clear reduced estimation uncertainty. (b) Noise variance vs. phase difference at a central node. Measurement noise variances are plotted in green for Sensor 1 and magenta for Sensor 3. Estimation variances, normalized to the SQL, for entangled (blue) and classical separable (red) sensor networks. Green and gold solid horizontal lines: theory curves for noise variances at two sensors. Solid black horizontal line: ideal estimation variance for entangled sensors; experimental deviation likely caused by imperfect phase locking between sensors. Dotted black horizontal line: the SQL for measurement noise variances and normalized estimation variances. While all classical data stay at the SQL, the estimation variances for the entangled sensor networks are sub-SQL and are significantly lower than the measurement noise variances at single sensors. Error bars reflect estimated measurement uncertainties caused by system instabilities.

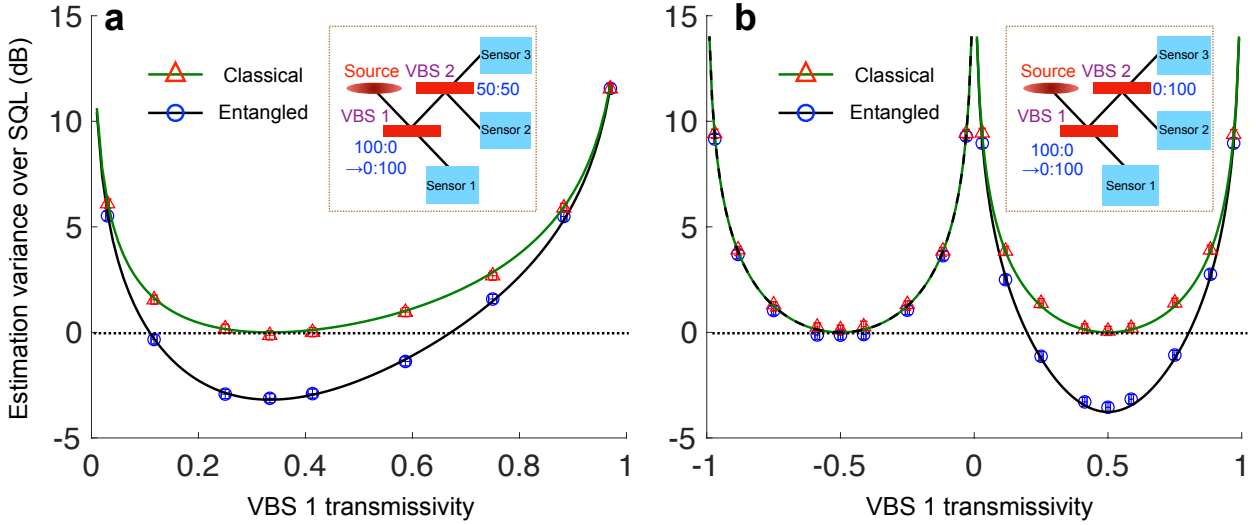

FIG. S7. Optimization of CV multipartite entangled state for the tasks of (a) estimating the average RF-field amplitude and (b) estimating the phase difference at a central node. Circles: entangled sensors data; triangles: classical separable sensors data; black curves: quantum theory; green curves: classical theory. Black horizontal dotted line: the SQL. Error bars account for estimated uncertainties arising from experimental instabilities. The symmetric classical curves vs. the asymmetric quantum curves in (b) manifests the correlated quantum noise arising from the homodyne detectors at different sensors. Insets: illustration of the tuning ranges of the VBS splitting ratios.

phase squeezed state at the source (shot-noise variance is  $1/4$ ) and  $1 - \eta$  being the overall loss seen by each sen-

sor.  $\delta_b = 0$  in the classical separable case and  $\delta_b < 0$  in the entangled case. The optimum parameter choices are thus  $w_m^{\text{opt}} = \sqrt{|c_m|} / \sqrt{\sum |c_m|}$  and  $g_m^{\text{opt}} = \text{sign}(c_m)$ , leading to a minimum estimation variance  $(\sum |c_m|)^2 \langle \text{Im}[\hat{b}]^2 \rangle / \beta^2$  (See Sec. I for derivation details).

The above result is used to model the experimental data in Fig. S7 and Fig. 5 of the main text. To facilitate the comparison, the minimum estimation variance of a classical separable sensor network,  $(\sum |c_m|)^2 / (4\beta^2)$ , is set as the SQL. In Fig. S6c, d, Fig. S7, and Figs. 4, 5 of the main text, the estimation variances are normalized to the SQL unit. The estimation of the average RF-field amplitude requires  $c_1 = c_2 = c_3 = 1/3$  and  $g_1 = g_2 = g_3 = 1$ . In the experiment, the splitting ratio of VBS 1,  $r$ , is tuned from 0:100 to 100:0 while the splitting ratio of VBS 2 is kept 50:50, so that  $w_1 = \sqrt{r}$ ,  $w_2 = w_3 = \sqrt{(1-r)/2}$ . This leads to  $\text{var} = (1/\beta^2)(\delta_b + [1/(1-r) + 1/4r]/9)$ , with the minimum achieved at  $r = 1/3$ . The theory and the experimental data are plotted in Fig. S7a, showing excellent agreement. To estimate the phase difference at a central node, we set  $c_1 = 1/2$ ,  $c_2 = 0$ ,  $c_3 = -1/2$ . The splitting ratio of VBS 1,  $r$ , is tuned between 100:0 and 0:100 while the splitting ratio of VBS 2 is kept 0:100, corresponding to  $w_1 = \sqrt{|r|}$ ,  $w_2 = 0$ ,  $w_3 = \sqrt{1-|r|}$  and  $g_1 = \text{sign}(r)$ ,  $g_2 = 1$ ,  $g_3 = -1$ . Here,  $g_m = -1$  indicates a  $\pi$ -phase shift on the RF field probed by the  $m$ -th sensor, which can be effectively viewed as applying a  $\pi$ -phase shift on its received entangled state while ensuring an unbiased estimator. For  $r > 0$ ,  $\text{var}_+ = (1/\beta^2)(\delta_b + [1/(1-r) + 1/r]/16)$ , which is minimized at  $r = 1/2$ , as seen in the right half of Fig. S7(b). We then set  $r < 0$ , leading to  $\text{var}_- = (1/\beta^2)[1/(1-|r|) + 1/|r|]/16$ . Since  $\delta_b$  is absent in  $\text{var}_-$ , the estimation variances for the entangled and classical separable cases are identical and are both minimized at  $r = -1/2$ , as shown in the left half of Fig. S7(b). The estimation of the phase difference at an edge node requires  $c_1 = 2$ ,  $c_2 = -3/2$ ,  $c_3 = -1/2$ . The splitting ratio of VBS 1 is kept 50:50 while the splitting ratio for VBS 2,  $r$ , is tuned between 100:0 and 0:100, corresponding to  $w_1 = \sqrt{1/2}$ ,  $w_2 = \sqrt{(1-|r|)/2}$ ,  $w_3 = \sqrt{|r|/2}$  and  $g_1 = 1$ ,  $g_2 = -1$ ,  $g_3 = -\text{sign}(r)$ . We first set  $r > 0$ , leading to  $\text{var}_+ = (1/\beta^2)(16\delta_b + [8 + 9/2(1-r) + 1/2r]/4)$ , which is plotted with the experimental data in the right half of Fig. 5 of the main text. The minimum estimation vari-

ance is achieved at  $r = 1/4$ . We then set  $r < 0$ , leading to  $\text{var}_- = (1/\beta^2)(9\delta_b + [8 + 9/2(1-|r|) + 1/2|r|]/4) > \text{var}_+$ , as plotted with the experimental data in the left half of Fig. 5 of the main text. The minimum estimation variance is achieved at  $r = -1/4$ .

### III. ENTANGLEMENT DISTRIBUTION

We have demonstrated an entangled sensor network in a free-space table-top experimental platform. For sensors spatially separated over a distance, low-loss optical fibers can be used to distributed the CV multipartite entanglement. State-of-the-art low-loss optical fibers have achieved 0.14 dB/km loss [S6], which will allow the entangled sensor network to achieve an appreciable quantum advantage over classical separable sensor networks over a few tens of kilometers. To show the feasibility of entanglement distribution, we simulated the performance of the entangled sensor network connected by low-loss optical fibers using the experimental parameters for the squeezing level, detector efficiency, and additional loss. The result is depicted in Fig. S8, showing a 2-dB (1-dB) estimation variance reduction for sensors 10 km (30 km) apart from the entanglement source. One interesting fact is that the entanglement-enhanced measurement sensitivity degrades at longer distances but never diminishes.

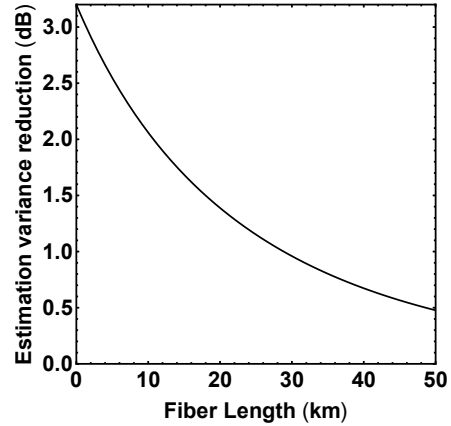

FIG. S8. Simulated estimation variance reduction in an entangled sensor network in which sensors are connected by low-loss optical fibers (0.14 dB/km).

- 
- [1] Q. Zhuang, Z. Zhang, and J. H. Shapiro, Distributed quantum sensing using continuous-variable multipartite entanglement, *Phys. Rev. A* **97**, 032329 (2018).
  - [2] W. Jiang *et al.*, Efficient bidirectional piezomechanical transduction between microwave and

optical frequency, arXiv:1909.04627.

- [3] Y. Xia, Q. Zhuang, W. Clark, and Z. Zhang, Repeater-enhanced distributed quantum sensing based on continuous-variable multipartite entanglement, *Phys. Rev. A* **99**, 012328 (2019).

- [4] M. Mehmet, S. Ast, T. Eberle, S. Steinlechner, H. Vahlbruch, and R. Schnabel, Squeezed light at 1550 nm with a quantum noise reduction of 12.3 dB, *Opt. Express* **19**, 25763 (2011).
- [5] K. Qian, Z. Eldredge, W. Ge, G. Pagano, C. Monroe, J. V. Porto, and A. V. Gorshkov, Heisenberg-scaling measurement protocol for analytic functions with quantum sensor networks, *Phys. Rev. A* **100**, 042304 (2019).
- [6] Y. Tamura, H. Sakuma, K. Morita, M. Suzuki, Y. Yamamoto, K. Shimada, Y. Honma, K. Sohma, T. Fujii, and T. Hasegawa, The First 0.14-dB/km Loss Optical Fiber and its Impact on Submarine Transmission, *J. Light. Technol.* **36**, 44–49 (2018).
